# Supplementary material for: Osmotic forces modify lipid membrane fluctuations
Source: arXiv:2510.10352 ancillary file (2026-02-21)
Supplement: Supplementary file 1 [file sahu-osmosis-flat-SM.pdf]

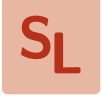

# Osmotic forces modify lipid membrane fluctuations

## Supplemental Material

AMARESH SAHU<sup>‡</sup>

*McKetta Department of Chemical Engineering,  
University of Texas, Austin TX 78712, USA*

This document is the supplemental material (SM) to the manuscript of the same name. In §1, we summarize the behavior of a lipid membrane in a general setting, following Sahu et al. (*Phys. Rev. E*, **96**, 2017) as well as Alkadri & Mandadapu (*Phys. Rev. E*, **112**, 2025). From here, the equations are specialized to the case of a planar bilayer with small out-of-plane undulations. Impermeable membranes are considered in §2, with the results extended to semipermeable membranes in §3. Our analysis of prior experiments is provided in §4.

### 1. The general governing equations

Consider an arbitrarily curved and deforming lipid membrane surface, surrounded by a solute-containing Newtonian fluid. Quantities above (resp. below) the membrane are labeled with a ‘plus’ (resp. ‘minus’) accent. In what follows, we present the equations governing the fluid, membrane, and solutes—as well as their interactions. None of the results in this section are new: the description of three-dimensional (3D) systems is well-known in the study of fluid mechanics and transport phenomena, while the membrane equations and coupling conditions were obtained in Refs. [1, 2].

#### 1.1. The bulk fluid

The fundamental unknowns describing an incompressible Newtonian fluid are the pressure field  $p^\pm$  and the velocity field  $\mathbf{v}^\pm$ . The corresponding governing equations are the continuity equation and local form of the balance of linear momentum, which for the fluid above and below the membrane are written as

$$\nabla \cdot \mathbf{v}^\pm = 0 \quad \text{and} \quad \rho_f \dot{\mathbf{v}}^\pm = \nabla \cdot \boldsymbol{\sigma}^\pm. \quad (1)$$

In Eq. (1)<sub>2</sub>,  $\rho_f$  is the fluid mass density and  $\dot{\mathbf{v}}$  is the fluid acceleration, or equivalently the material time derivative of the velocity:  $\dot{\mathbf{v}} = \partial \mathbf{v} / \partial t + (\nabla \mathbf{v}) \mathbf{v}$ . The stress tensor  $\boldsymbol{\sigma}^\pm$  for a Newtonian fluid is given by

$$\boldsymbol{\sigma}^\pm = -p^\pm \mathbf{I} + \mu_f \left[ (\nabla \mathbf{v}^\pm) + (\nabla \mathbf{v}^\pm)^T \right], \quad (2)$$

where the fluid shear viscosity  $\mu_f$  is assumed to be the same above and below the membrane. Upon substituting Eq. (2) into Eq. (1)<sub>2</sub> and simplifying with Eq. (1)<sub>1</sub>, we obtain

$$\rho_f \dot{\mathbf{v}}^\pm = \mu_f \nabla^2 \mathbf{v}^\pm - \nabla p^\pm. \quad (3)$$

Equation (3) is the well-known Navier–Stokes equation, which along with Eq. (1)<sub>1</sub> can be used to solve for the velocity and pressure fields in the fluid.

---

<sup>‡</sup>[asahu@che.utexas.edu](mailto:asahu@che.utexas.edu)

### 1.2. The osmolyte species

The fundamental unknown describing the osmolyte species is the concentration field  $c^\pm$ . The well-known diffusion equation governs the evolution of the solute concentration over time, and is written as

$$\frac{\partial c^\pm}{\partial t} + \mathbf{v}^\pm \cdot \nabla c^\pm = -\nabla \cdot \mathbf{j}^\pm, \quad \text{where} \quad \mathbf{j}^\pm = -D \nabla c^\pm \quad (4)$$

is the diffusive concentration flux. In Eq. (4)<sub>2</sub>,  $D$  is the solute diffusion constant, which is assumed to be the same on both sides of the membrane. By substituting Eq. (4)<sub>2</sub> into Eq. (4)<sub>1</sub>, we obtain

$$\frac{\partial c^\pm}{\partial t} + \mathbf{v}^\pm \cdot \nabla c^\pm = D \nabla^2 c^\pm, \quad (5)$$

which is a single equation for the concentration field  $c^\pm$ .

### 1.3. The lipid membrane

The fundamental unknowns describing an arbitrarily curved and deforming lipid membrane are the velocity field  $\mathbf{v}$  and the surface tension field  $\lambda$ . Both quantities are defined only on the membrane surface, whose position is denoted  $\mathbf{x}$ . It is useful to decompose the membrane velocity field as

$$\mathbf{v} = v^\alpha \mathbf{a}_\alpha + v \mathbf{n}, \quad (6)$$

where a detailed account of membrane geometry, kinematics, and dynamics are provided in Ref. [1]. We briefly mention that (i) ‘ $\alpha$ ’ and other Greek indices span the set  $\{1, 2\}$  and denote independent directions on the membrane surface, (ii) summation is implied over repeated indices, (iii)  $\mathbf{a}_\alpha$  are in-plane vectors that form a basis of the plane tangent to the surface, and (iv)  $\mathbf{n}$  is the unit normal to the membrane, which points into the fluid region above the membrane labeled with a ‘plus’ accent.

With Eq. (6), one can treat  $v^\alpha$ ,  $v$ , and  $\lambda$  as the four fundamental membrane unknowns. The corresponding governing equations are the continuity equation, two in-plane equations, and shape (or out-of-plane) equation—respectively given by

$$v^\alpha_{;\alpha} - 2vH = 0, \quad (7)$$

$$a^{\alpha\beta} \lambda_{,\beta} + \pi^\beta_{;\beta} + f^\alpha = 0, \quad (8)$$

and

$$f + 2\lambda H + \pi^{\alpha\beta} b_{\alpha\beta} - 2k_b H(H^2 - K) - k_b \Delta_s H = 0. \quad (9)$$

In the membrane equations, we introduce the following notation: (i)  $(\cdot)_{;\alpha}$  denotes the covariant derivative in the ‘ $\alpha$ ’ direction, (ii)  $a^{\alpha\beta}$  is the contravariant metric, which describes distances on the membrane surface, (iii)  $\pi^{\alpha\beta} = \pi^{\beta\alpha}$  are the in-plane viscous stresses, (iv)  $b_{\alpha\beta}$  are the components of the curvature tensor, (v)  $k_b$  is the bending modulus of the membrane, (vi)  $H$  is the mean curvature, (vii)  $K$  is the Gaussian curvature, and (viii)  $\Delta_s$  denotes the surface Laplacian operator, where  $\Delta_s(\cdot) := a^{\alpha\beta}(\cdot)_{;\alpha\beta}$ . In addition,  $\mathbf{f}$  is the total force acting on the membrane, which is decomposed into in-plane and out-of-plane components as

$$\mathbf{f} = f^\alpha \mathbf{a}_\alpha + f \mathbf{n}. \quad (10)$$

### 1.4. The coupling conditions

To close our mathematical description of the general governing equations, we require coupling conditions at the membrane surface. To begin, we recognize the force exerted on the membrane by the surrounding fluid is given by

$$\mathbf{f} = (\boldsymbol{\sigma}^+ - \boldsymbol{\sigma}^-) \mathbf{n} = \llbracket \boldsymbol{\sigma} \rrbracket \mathbf{n} , \quad (11)$$

where  $\llbracket (\cdot) \rrbracket := (\cdot)^+ - (\cdot)^-$  denotes the jump in a quantity at the membrane surface. Next, we assume there is no in-plane slip between the membrane and fluid velocities, written as

$$\mathbf{v} \cdot \mathbf{a}_\alpha = \mathbf{v}^\pm \cdot \mathbf{a}_\alpha . \quad (12)$$

Although the bulk velocity field must be continuous, such that at the membrane surface

$$\mathbf{v}^+ \cdot \mathbf{n} = \mathbf{v}^- \cdot \mathbf{n} , \quad (13)$$

these velocities need not be equal to the out-of-plane membrane velocity if fluid can pass through the membrane. The relationship between the membrane and bulk velocities in the out-of-plane direction was obtained in Ref. [2], which studied the coupled system by applying the concepts of irreversible thermodynamics within a differential geometric setting. Their result can be written as

$$\mathbf{f} \cdot \mathbf{n} + k_B \theta \llbracket c \rrbracket = \kappa (\mathbf{v}^\pm - \mathbf{v}) \cdot \mathbf{n} , \quad (14)$$

where  $k_B \theta$  is the thermal energy. The membrane impermeability  $\kappa$  is the transport coefficient for water flow through the membrane, with  $\kappa \rightarrow \infty$  in the limit of an impermeable membrane. Finally, we assume the membrane is ideally selective, for which fluid can pass through the membrane while solutes cannot. In this limit, we require the sum of the diffusive and convective fluxes of solute normal to the membrane to be zero—expressed as

$$\left[ \mathbf{j}^\pm + c^\pm (\mathbf{v}^\pm - \mathbf{v}) \right] \cdot \mathbf{n} = 0 . \quad (15)$$

With Eqs. (11)–(15), our coupled description of the membrane and its surroundings is mathematically well-posed.

## 2. The impermeable membrane surrounded by fluid

Consider a fluctuating, nearly planar, impermeable lipid membrane surrounded by fluid. The stationary base state is captured by the quantities

$$h_{(0)} = 0 , \quad v_\alpha^{(0)} = 0 , \quad \lambda_{(0)} = \lambda_c , \quad v_j^\pm = 0 , \quad \text{and} \quad p_{(0)}^\pm = p_c , \quad (16)$$

where the characteristic base tension  $\lambda_c$  and pressure  $p_c$  are known constants, and Roman indices span  $\{1, 2, 3\}$ . Perturbed (or fluctuating) quantities are described with a ‘tilde’ in the SM (though not the main text). In this case, we have

$$h = \tilde{h} , \quad v_\alpha = \tilde{v}_\alpha , \quad \lambda = \lambda_c + \tilde{\lambda} , \quad v_j^\pm = \tilde{v}_j^\pm , \quad \text{and} \quad p^\pm = p_c + \tilde{p}^\pm . \quad (17)$$

### 2.1. The fluid solution

The perturbed fluid is governed by the incompressibility constraint and time-dependent Stokes equation, respectively given by

$$\tilde{v}_{j,j}^{\pm} = 0 \quad \text{and} \quad \rho_f \tilde{v}_{j,t}^{\pm} = \mu_f \tilde{v}_{j,kk}^{\pm} - \tilde{p}_{,j}^{\pm} . \quad (18)$$

Here and from now on, the summation convention is assumed over repeated Roman indices. At this point all fluid unknowns are decomposed into normal modes as

$$\tilde{p}^{\pm}(x, y, z, t) = \sum_{\mathbf{q}} \hat{p}_{\mathbf{q}}^{\pm}(z) \exp [i(q_x x + q_y y) - \omega_{\mathbf{q}} t] \quad (19)$$

and

$$\tilde{v}_j^{\pm}(x, y, z, t) = \sum_{\mathbf{q}} \hat{v}_{j\mathbf{q}}^{\pm}(z) \exp [i(q_x x + q_y y) - \omega_{\mathbf{q}} t] . \quad (20)$$

Taking the divergence of the Stokes equation and applying the continuity equation reveals that the pressure field is harmonic:  $\tilde{p}_{,jj}^{\pm} = 0$ . Substituting the normal mode decomposition yields

$$\frac{d^2 \hat{p}_{\mathbf{q}}^{\pm}}{dz^2} = q^2 \hat{p}_{\mathbf{q}}^{\pm} , \quad \text{for which} \quad \hat{p}_{\mathbf{q}}^{\pm} = \bar{p}_{\mathbf{q}}^{\pm} e^{\mp q z} . \quad (21)$$

In Eq. (21), we assume the perturbed pressure decays infinitely far from the membrane surface, and  $\bar{p}_{\mathbf{q}}^{\pm}$  are integration constants to be determined via boundary conditions. The pressure solution is treated as a forcing term in the Stokes equation. Following §94 of Ref. [3], the (complex) modified wavenumber  $k_{\nu}$  is defined via the relations

$$k_{\nu}^2 := q^2 - \frac{\omega_{\mathbf{q}}}{\nu_f} , \quad \text{where} \quad \nu_f := \frac{\mu_f}{\rho_f} \quad \text{and} \quad \text{Re}\{k_{\nu}\} \geq 0 \quad (22)$$

by construction. We find the in-plane and out-of-plane fluid equations—in terms of normal modes—to respectively be expressed as

$$\frac{d^2 \hat{v}_{\alpha\mathbf{q}}^{\pm}}{dz^2} = k_{\nu}^2 \hat{v}_{\alpha\mathbf{q}}^{\pm} + \frac{i q_{\alpha} \bar{p}_{\mathbf{q}}^{\pm}}{\mu_f} e^{\mp q z} \quad \text{and} \quad \frac{d^2 \hat{v}_{z\mathbf{q}}^{\pm}}{dz^2} = k_{\nu}^2 \hat{v}_{z\mathbf{q}}^{\pm} \mp \frac{q \bar{p}_{\mathbf{q}}^{\pm}}{\mu_f} e^{\mp q z} . \quad (23)$$

It is straightforward to verify that the solutions to Eq. (23) are given by

$$\hat{v}_{\alpha\mathbf{q}}^{\pm} = \bar{v}_{\alpha\mathbf{q}}^{\pm} e^{\mp k_{\nu} z} + \frac{i q_{\alpha} \bar{p}_{\mathbf{q}}^{\pm}}{\mu_f (q^2 - k_{\nu}^2)} e^{\mp q z} \quad \text{and} \quad \hat{v}_{z\mathbf{q}}^{\pm} = \bar{v}_{z\mathbf{q}}^{\pm} e^{\mp k_{\nu} z} \mp \frac{q \bar{p}_{\mathbf{q}}^{\pm}}{\mu_f (q^2 - k_{\nu}^2)} e^{\mp q z} , \quad (24)$$

where  $\bar{v}_{\alpha\mathbf{q}}^{\pm}$  and  $\bar{v}_{z\mathbf{q}}^{\pm}$  are constants of integration that will be determined subsequently.

### 2.2. The conditions coupling the membrane and fluid

With the generic form of the fluid solution, we seek to determine the relationship between membrane and fluid unknowns. We begin by decomposing all membrane variables in terms of normal modes as

$$\tilde{\lambda}(x, y, t) = \sum_{\mathbf{q}} \hat{\lambda}_{\mathbf{q}} \exp [i(q_x x + q_y y) - \omega_{\mathbf{q}} t] , \quad (25)$$

$$\tilde{h}(x, y, t) = \sum_{\mathbf{q}} \hat{h}_{\mathbf{q}} \exp [i(q_x x + q_y y) - \omega_{\mathbf{q}} t] , \quad (26)$$

and

$$\tilde{v}_{\alpha}(x, y, t) = \sum_{\mathbf{q}} \hat{v}_{\alpha\mathbf{q}} \exp [i(q_x x + q_y y) - \omega_{\mathbf{q}} t] . \quad (27)$$

The no-slip condition at the membrane surface requires  $\tilde{h}_{,t} = \tilde{v}_{z=0}^{\pm}|_{z=0}$ , for which

$$-\omega_{\mathbf{q}} \hat{h}_{\mathbf{q}} = \bar{v}_{z\mathbf{q}}^{\pm} \mp \frac{q \bar{p}_{\mathbf{q}}^{\pm}}{\mu_{\text{f}}(q^2 - k_{\nu}^2)} . \quad (28)$$

Furthermore, the requirement that both the membrane and the surrounding fluid are incompressible requires  $\tilde{v}_{z,z}^{\pm}|_{z=0} = 0$ , which yields

$$\bar{v}_{z\mathbf{q}}^{\pm} = \pm \frac{q^2 \bar{p}_{\mathbf{q}}^{\pm}}{k_{\nu} \mu_{\text{f}}(q^2 - k_{\nu}^2)} . \quad (29)$$

By substituting Eq. (29) into Eq. (28) and rearranging terms, we find the membrane height and fluid pressure are related according to

$$\bar{p}_{\mathbf{q}}^{\pm} = \mp \frac{\mu_{\text{f}} \nu_{\text{f}} k_{\nu}}{q} (q^2 - k_{\nu}^2) (q + k_{\nu}) \hat{h}_{\mathbf{q}} . \quad (30)$$

The in-plane components of the no-slip condition are similarly obtained as

$$\hat{v}_{\alpha\mathbf{q}} = \bar{v}_{\alpha\mathbf{q}}^{\pm} + \frac{i q_{\alpha} \bar{p}_{\mathbf{q}}^{\pm}}{\mu_{\text{f}}(q^2 - k_{\nu}^2)} . \quad (31)$$

### 2.3. The membrane solution and dispersion relation

At this point, we turn to the perturbed membrane equations to solve for the dynamics of the system. The linearized continuity, shape, and in-plane equations about a flat patch are respectively given by [4]

$$\tilde{v}_{\alpha,\alpha} = 0 , \quad (32)$$

$$\rho_{\text{m}} \tilde{h}_{,tt} = \lambda_{\text{c}} \tilde{h}_{,\alpha\alpha} - \frac{k_{\text{b}}}{2} \tilde{h}_{,\alpha\alpha\beta\beta} - \tilde{p}^{+} + \tilde{p}^{-} , \quad (33)$$

and

$$\rho_{\text{m}} \tilde{v}_{\alpha,t} = \zeta \tilde{v}_{\alpha,\beta\beta} + \tilde{\lambda}_{,\alpha} + \mu_{\text{f}} (\tilde{v}_{\alpha,z}^{+} + \tilde{v}_{z,\alpha}^{+} - \tilde{v}_{\alpha,z}^{-} - \tilde{v}_{z,\alpha}^{-}) , \quad (34)$$

where all fluid quantities are evaluated at  $z = 0$ : the location of the unperturbed membrane surface. Note that in Eq. (33), we omit the normal viscous forces because they are identically zero (recall  $\tilde{v}_{z,z}^{\pm}|_{z=0} = 0$ ). In terms of normal modes, the continuity equation (32) is expressed as  $i q_{\alpha} \hat{v}_{\alpha\mathbf{q}} = 0$ , which requires  $q_x \hat{v}_{x\mathbf{q}} = -q_y \hat{v}_{y\mathbf{q}}$ . The shape equation (33) is expressed in terms of normal modes as

$$\rho_{\text{m}} \omega_{\mathbf{q}}^2 \hat{h}_{\mathbf{q}} = -E \hat{h}_{\mathbf{q}} - \bar{p}_{\mathbf{q}}^{+} + \bar{p}_{\mathbf{q}}^{-} , \quad (35)$$

where  $E := \lambda_{\text{c}} q^2 + \frac{1}{2} k_{\text{b}} q^4$  as introduced in the main text. Substituting Eq. (30) into Eq. (35) yields an equation in which every terms is linear in  $\hat{h}_{\mathbf{q}}$ . Assuming a nontrivial solution, for which  $\hat{h}_{\mathbf{q}} \neq 0$ , and then substituting Eq. (22)<sub>1</sub> yields

$$\rho_{\text{m}} \nu_{\text{f}}^2 (q^2 - k_{\nu}^2)^2 - \frac{2 \mu_{\text{f}} \nu_{\text{f}} k_{\nu}}{q} (q^2 - k_{\nu}^2) (q + k_{\nu}) + E = 0 , \quad (36)$$

which is a fourth-order polynomial for  $k_\nu$ . Since we require the real part of  $k_\nu$  to be positive by construction, only two solutions are valid—and can be understood by drawing analogy to a classical spring–mass–damper system. Our code to solve Eq. (36) for physical  $k_\nu$ , with  $\text{Re}\{k_\nu\} \geq 0$ , and determine the corresponding  $\omega_q$  is provided at [github.com/sahu-lab/osmosis-flat](https://github.com/sahu-lab/osmosis-flat).

#### 2.4. The trivial in-plane solution

The in-plane equations (34) were not used to obtain Eq. (36). To probe the in-plane dynamics, we express Eq. (34) in terms of normal modes—and substitute the fluid solution (24)—to obtain

$$-\rho_m \omega_q \hat{v}_{\alpha q} = -q^2 \zeta \hat{v}_{\alpha q} + i q_\alpha \hat{\lambda}_q + i q_\alpha \mu_f (\bar{v}_{zq}^+ - \bar{v}_{zq}^-) - k_\nu \mu_f (\bar{v}_{\alpha q}^+ + \bar{v}_{\alpha q}^-) - \frac{2i q_\alpha q}{q^2 - k_\nu^2} (\bar{p}_q^+ + \bar{p}_q^-). \quad (37)$$

From Eq. (30), we recognize  $\bar{p}_q^+ + \bar{p}_q^- = 0$ . Equation (29) then reveals  $\bar{v}_{zq}^+ - \bar{v}_{zq}^- = 0$ , while Eq. (31) requires  $2\hat{v}_{\alpha q} = \bar{v}_{\alpha q}^+ + \bar{v}_{\alpha q}^-$ . With these results, Eq. (38) simplifies to

$$-\rho_m \omega_q \hat{v}_{\alpha q} = -q^2 \zeta \hat{v}_{\alpha q} + i q_\alpha \hat{\lambda}_q - 2k_\nu \mu_f \hat{v}_{\alpha q}. \quad (38)$$

Taking the divergence of Eq. (38) and applying the continuity equation  $i q_\alpha \hat{v}_{\alpha q} = 0$  reveals

$$\hat{\lambda}_q = 0. \quad (39)$$

With Eq. (39), Eq. (38) simplifies to a form where every term is linear in  $\hat{v}_{\alpha q}$ . If we assume a nontrivial solution ( $\hat{v}_{\alpha q} \neq 0$ ) and substitute Eq. (22)<sub>1</sub> for  $\omega_q$ , we find

$$\rho_m \nu_f k_\nu^2 + 2\mu_f k_\nu + q^2 (\zeta - \nu_f \rho_m) = 0. \quad (40)$$

Note that for typical fluid and membrane parameters, all three coefficients in the quadratic equation for  $k_\nu$  are positive—and so all solutions involve  $k_\nu$  either being negative, or having a negative real part. Thus, there are no physical solutions  $k_\nu$  for the in-plane dynamics.

### 3. The semipermeable membrane surrounded by solutes and fluid

The stationary base state of the semipermeable scenario is given by Eq. (16), along with a uniform concentration field

$$c_{(0)}^\pm = c_0 \quad (41)$$

for known, constant  $c_0$ . The concentration of the perturbed system is given by  $c^\pm = c_0 + \tilde{c}^\pm$ , where the ‘tilde’ accent is once again only used in the SM [cf. Eq. (17)].

#### 3.1. The solute concentration profile

The time evolution of the perturbed concentration  $\tilde{c}^\pm$  is given by the diffusion equation

$$\tilde{c}_{,t}^\pm = D \tilde{c}_{,jj}^\pm, \quad (42)$$

where  $D$  is the solute diffusion constant in the surrounding fluid at infinite dilution. When the perturbed concentration is decomposed into normal modes as

$$\tilde{c}^\pm(x, y, z, t) = \sum_q \hat{c}_q^\pm(z) \exp[i(q_x x + q_y y) - \omega_q t], \quad (43)$$

the diffusion equation (42) simplifies to

$$\frac{d^2 \hat{c}_q^\pm}{dz^2} = k_D^2 \hat{c}_q^\pm, \quad \text{where} \quad k_D^2 := q^2 - \frac{\omega q}{D} \quad \text{and} \quad \text{Re}\{k_D\} \geq 0 \quad (44)$$

by construction [cf. Eq. (22)]. With the assumption that concentration fluctuations decay infinitely far from the membrane surface, the concentration solution is expressed as

$$\hat{c}_q^\pm = \bar{c}_q^\pm e^{\mp k_D z}, \quad (45)$$

where  $\bar{c}_q^\pm$  are two integration constants that will be determined from the boundary and coupling conditions.

### 3.2. The conditions coupling the membrane, fluid, and solutes

When the lipid membrane is semipermeable, fluid passes through the membrane while solutes do not. The linearized equations governing both phenomena were recently found to be [2]

$$-D\tilde{c}_{,z}^\pm + c_0(\tilde{v}_z^\pm - \tilde{h}_{,t}) = 0 \quad \text{and} \quad \kappa(\tilde{v}_z^\pm - \tilde{h}_{,t}) = k_B\theta(\tilde{c}^+ - \tilde{c}^-) - (\tilde{p}^+ - \tilde{p}^-), \quad (46)$$

where  $\kappa$  is the membrane impermeability. In addition, the  $z$ -component of the fluid velocity field is assumed continuous at the membrane surface—though it may differ from the membrane velocity  $\tilde{h}_{,t}$ . With the continuity of  $v_z^\pm$  at  $z = 0$ , as well as Eq. (29), we find (note the general fluid solution in §2.1 remains valid)

$$\bar{p}_q^+ = -\bar{p}_q^- \quad \text{and} \quad \bar{v}_{zq}^+ = \bar{v}_{zq}^-. \quad (47)$$

We also find the no-flux condition (46)<sub>1</sub> requires  $\tilde{c}_{,z}^+ = \tilde{c}_{,z}^-$ , for which

$$\bar{c}_q^+ = -\bar{c}_q^-. \quad (48)$$

Accordingly, the fluid pressure,  $z$ -component of the fluid velocity, and solute concentration can all be expressed in terms of  $\bar{p}_q^+$ ,  $\bar{v}_{zq}^+$ , and  $\bar{c}_q^+$ . We do not consider the in-plane fluid behavior, as it led to a trivial solution in the impermeable scenario.

### 3.3. The membrane solution and dispersion relation

The membrane equations (32)–(34) are unchanged in the presence of solutes in the surrounding fluid, as found in Ref. [2]. To determine the dispersion relation from Eq. (35), we require the relationship between  $\hat{h}_q$  and  $\bar{p}_q^+$ . To this end, we combine the no-flux condition and permeability equation (46) to obtain  $\kappa D\tilde{c}_{,z}^+/c_0 = k_B\theta(\tilde{c}^+ - \tilde{c}^-) - (\tilde{p}^+ - \tilde{p}^-)$ , which is expressed in terms of normal modes as

$$-\frac{\kappa D k_D}{c_0} \bar{c}_q^+ = 2k_B\theta \bar{c}_q^+ - 2\bar{p}_q^+. \quad (49)$$

With Eq. (49),  $\bar{c}_q^+$  can be expressed in terms of  $\bar{p}_q^+$ . Next, we examine the Fourier representation of the no-flux condition (46)<sub>1</sub> after the concentration (45) and fluid velocity (24) solutions are substituted:

$$\frac{D k_D \bar{c}_q^+}{c_0} + \bar{v}_{zq}^+ - \frac{q \bar{p}_q^+}{\mu_t(q^2 - k_\nu^2)} + \omega_q \hat{h}_q = 0. \quad (50)$$

By then substituting Eq. (29) into Eq. (50),<sup>‡</sup> we obtain a relation involving only  $\bar{c}_q^+$ ,  $\bar{p}_q^+$ , and  $\hat{h}_q$ . Thus, along with Eq. (49), we find  $\hat{h}_q$  and  $\bar{p}_q^+$  are related according to

$$\bar{p}_q^+ = \frac{-\omega_q \hat{h}_q}{\frac{2Dk_D}{2k_B\theta c_0 + \kappa Dk_D} + \left(\frac{q}{k_\nu} - 1\right) \frac{q}{\mu_f(q^2 - k_\nu^2)}}. \quad (51)$$

Substituting Eqs. (51) and (47)<sub>1</sub> into Eq. (35) yields an equation where every term is proportional to  $\hat{h}_q$ . Assuming a nontrivial solution ( $\hat{h}_q \neq 0$ ), we arrive at the dispersion relation

$$\rho_m \omega_q^2 + q^2 \lambda_c + q^4 \frac{k_b}{2} - \frac{2\omega_q}{\frac{2Dk_D}{2k_B\theta c_0 + \kappa Dk_D} + \left(\frac{q}{k_\nu} - 1\right) \frac{q}{\mu_f(q^2 - k_\nu^2)}} = 0. \quad (52)$$

Note that Eq. (52) is an implicit equation for  $\omega_q$ , as both  $k_\nu$  (22) and  $k_D$  (44) depend on  $\omega_q$  as well.

### 3.3.1. The method of numerical solution

Equation (52) is a nonlinear equation for  $\omega_q$ , for which numerical solvers generally (i) require an initial guess and (ii) provide a single nearby solution. Rather than having to search for a set of good initial guesses, we instead choose to manipulate Eq. (52) into a polynomial equation for  $k_\nu$ . Before doing so, it is convenient to define the parameter  $\alpha$  as

$$\alpha := \frac{k_B\theta c_0}{D}. \quad (53)$$

The dispersion relation (52) can then be expressed as either

$$\rho_m \omega_q^2 + E - \frac{2\omega_q}{\frac{1}{(\alpha/k_D) + (\kappa/2)} + \left(\frac{q}{k_\nu} - 1\right) \frac{q}{\rho_f \omega_q}} = 0 \quad (54)$$

or

$$\rho_m \omega_q^2 + E - \frac{2\omega_q}{\frac{1}{(\alpha/k_D) + (\kappa/2)} + \frac{q}{\mu_f k_\nu (q + k_\nu)}} = 0. \quad (55)$$

By algebraically manipulating Eq. (55) and expressing  $k_D$  in terms of  $k_\nu$ , we obtain a 14<sup>th</sup>-order polynomial equation for  $k_\nu$ . Our code to determine the frequencies  $\omega_q$  as a function of  $q$ , with physical  $k_\nu$  and  $k_D$ , is provided at [github.com/sahu-lab/osmosis-flat](https://github.com/sahu-lab/osmosis-flat).

### 3.3.2. An approximate dispersion relation

Recall that the membrane is nearly impermeable, as reflected by  $\kappa$  being large and the permeability number  $\mathcal{P} := \mu_f q / \kappa$  being small. In what follows, we seek to understand how a small but nonzero  $\mathcal{P}$  can significantly affect the behavior of the coupled membrane–solute–fluid system. To this end, Eq. (55) is Taylor expanded about  $\kappa^{-1} = 0$  to yield

$$\rho_m \omega_q^2 + E - \frac{2\omega_q \mu_f k_\nu}{q} (q + k_\nu) \left[ 1 - \frac{2\mu_f k_\nu (q + k_\nu)}{\kappa q} \left( 1 - \frac{2\alpha}{\kappa k_D} \right) \right] = 0. \quad (56)$$

---

<sup>‡</sup>Equation (29) is valid in the semipermeable setting, since the membrane and fluid each remain incompressible.

If  $\kappa$  were set to  $\infty$ , then Eq. (56) would simplify to the impermeable dispersion relation (36)—which is now known to be approximated by  $\rho_{\text{eff}} \omega_{\mathbf{q}}^2 - 4\mu_{\text{f}} q \omega_{\mathbf{q}} + E = 0$ . We posit that the fluid inertia will be approximately accounted for upon changing  $\{\rho_{\text{m}}, k_{\nu}\}$  to  $\{\rho_{\text{eff}}, q\}$  in Eq. (56). The resulting approximate equation is given by

$$\rho_{\text{eff}} \omega_{\mathbf{q}}^2 + E - 4\mu_{\text{f}} q \omega_{\mathbf{q}} \left[ 1 - \frac{4\mu_{\text{f}} q}{\kappa} \left( 1 - \frac{2\alpha}{\kappa k_D} \right) \right] = 0. \quad (57)$$

Again, since the membrane is nearly impermeable, the  $k_D$  appearing in Eq. (57) can be approximated by substituting the impermeable frequency  $\omega_{\mathbf{q}}^{\text{imp}}$  into Eq. (44)<sub>2</sub>. In what follows, we separately consider the case where  $\omega_{\mathbf{q}}^{\text{imp}} > \tilde{\omega}_D$ , as is the case for the inertial branch and the membrane branch outside the dome, and the case where  $\omega_{\mathbf{q}}^{\text{imp}} < \tilde{\omega}_D$ , which is satisfied for the membrane branch inside the dome.

**The case where diffusion is slow.**—Following Eq. (13) of the main text, for  $k_D = \mp i q \tilde{\eta}$  we have  $\hat{c}_{\mathbf{q}}^+ = \bar{c}_{\mathbf{q}}^+ e^{\pm i q \tilde{\eta} z}$  and  $\hat{c}_{\mathbf{q}}^- = \bar{c}_{\mathbf{q}}^- e^{\mp i q \tilde{\eta} z}$ . Equation (57) can then be written in terms of  $\mathcal{P}$  and the osmotic number  $\mathcal{S} := k_{\text{B}} \theta c_0 / (D \kappa q) = \alpha / (\kappa q)$  as

$$\rho_{\text{eff}} \omega_{\mathbf{q}}^2 + E - 4\mu_{\text{f}} q \omega_{\mathbf{q}} (1 - 4\mathcal{P}) = \pm \frac{8i\mathcal{P}\mathcal{S}}{\tilde{\eta}} (4\mu_{\text{f}} q) \omega_{\mathbf{q}}. \quad (58)$$

In Eq. (58), the in-phase change to the drag is of order  $\mathcal{P}$ , and can be neglected—resulting in Eq. (14) of the main text.

**The case where diffusion is fast.**—On the membrane branch inside the dome,  $\tilde{\omega}_D > \omega_{\mathbf{q}}^{\text{imp}}$ . To lowest order in the permeability number  $\mathcal{P}$ , we find  $k_D = q(1 - \omega_{\mathbf{q}}^{\text{imp}}/\tilde{\omega}_D)^{1/2} \in \mathbb{R}^+$  and  $\hat{c}_{\mathbf{q}}^{\pm} = \bar{c}_{\mathbf{q}}^{\pm} e^{\mp k_D z}$ : an exponentially decaying, physically meaningful concentration field. The in-phase corrections to Eq. (57) are negligible, and the frequency  $\omega_{\mathbf{q}}$  is approximately equal to its impermeable counterpart.

#### 4. The analysis of relevant experiments

This section details how the data in Fig. 5 of the main text was collected. The raw data from prior studies, as well as all processing scripts, is shared at [github.com/sahu-lab/osmosis-flat](https://github.com/sahu-lab/osmosis-flat). Data was collected from published figures using the online tool [apps.automeris.io/wpd4](https://apps.automeris.io/wpd4). Our analysis of experimental data is based on the description in Ref. [5]. More precisely, suppose the instantaneous radial profile  $r(\varphi, t)$  of the vesicle's equatorial cross-section is given by [5, Eq. (8)]

$$r(\varphi, t) = r_{\text{v}}(t) \left[ 1 + \sum_{m=1}^{m_{\text{max}}} \left( a_m \cos(m\varphi) + b_m \sin(m\varphi) \right) \right], \quad (59)$$

where  $\varphi$  is the azimuthal angle,  $r_{\text{v}}(t)$  is the instantaneous vesicle radius, and  $r_{\text{v}} := \langle r_{\text{v}}(t) \rangle$  is the average vesicle radius. Radial contour fluctuations are then expected to satisfy [5, Eqs. (11), (14)]

$$\frac{\pi r_{\text{v}}^3}{2} \left( \langle c_m^2 \rangle - \langle c_m \rangle^2 \right) = \frac{k_{\text{B}} \theta}{2\lambda_{\text{c}}} \left( \frac{1}{q_x} - \frac{1}{\sqrt{q_x^2 + 2\lambda_{\text{c}}/k_{\text{b}}}} \right), \quad \text{where } c_m := \sqrt{a_m^2 + b_m^2} \quad (60)$$

for  $m = q_x r_{\text{v}}$ . The right-hand side of Eq. (60) is the  $y$ -axis of Fig. 5 in the main text:  $\ell_{\text{c}} \langle |\tilde{h}_{q_x}|^2 \rangle$ . We now aggregate experimental measurements of the left-hand side of Eq. (60) from prior studies.

***Analysis of Faizi et al. (Soft Matter, 2020)***

In Faizi et al. [6], the instantaneous radial profile of the vesicle cross-section is decomposed into Fourier modes as

$$r(\varphi, t) = r_v \left( 1 + \sum_{m=-m_{\max}}^{m_{\max}} \hat{u}_m(t) e^{im\varphi} \right), \quad (61)$$

where the coefficients  $\hat{u}_m$  are complex. In comparing Eqs. (59) and (61), we find

$$\hat{u}_0(t) = \frac{r_v(t)}{r_v} - 1, \quad \hat{u}_m = (a_m - ib_m) \frac{r_v(t)}{2r_v}, \quad \text{and} \quad \hat{u}_{-m} = (a_m + ib_m) \frac{r_v(t)}{2r_v}. \quad (62)$$

Consequently,  $4\langle |\hat{u}_m^2| \rangle = \langle c_m^2 \rangle - \langle c_m \rangle^2$ , and Eq. (60) can be expressed as

$$2\pi r_v^3 \langle |\hat{u}_m^2| \rangle = \frac{k_B \theta}{2\lambda_c} \left( \frac{1}{q_x} - \frac{1}{\sqrt{q_x^2 + 2\lambda_c/k_b}} \right). \quad (63)$$

In Fig. 1 of Ref. [6],  $\langle |\hat{u}_m^2| \rangle$  is plotted as a function of  $m$ . We scale their  $x$ -axis by  $1/r_v$  and their  $y$ -axis by  $2\pi r_v^3$  to generate the corresponding data in Fig. 5 of the main text, where we approximate  $r_v \approx 3 \cdot 10^4$  nm from their inset to Fig. 1.

***Analysis of Rautu et al. (Soft Matter, 2017)***

While Rautu et al. [7] investigates how optical projection affects the observed radial contour fluctuations, we interpret the data in Fig. 2(a) as the amplitudes  $\langle |\hat{u}_m^2| \rangle$  [cf. Eq. (61)]. Accordingly, we scale their  $x$ -axis by  $1/r_v$  and their  $y$ -axis by  $2\pi r_v^3$ .

***Analysis of Pécrcéaux et al. (Eur. Phys. J. E, 2004)***

The analysis of radial vesicle fluctuations by Pécrcéaux et al. [5] is fundamental to our own understanding. In Fig. 6 of their work, experimental data is presented as in Fig. 5 of the main text of the present study. No scaling of the data is required.

***Analysis of Park et al. (Soft Matter, 2022)***

In Park et al. [8], vesicles containing many motile bacteria are analyzed. Such vesicles exhibit enhanced long-wavelength fluctuations, while shorter-wavelength modes are unchanged. We extract the unaltered fluctuation data from Fig. 6(c). In doing so, we found there is a  $1/r_v$  discrepancy between the plotted modes and theoretical fit, when  $r_v$  is measured in microns. Though their  $y$ -axis is labeled (in our notation) as  $\ell_c \langle |\tilde{h}_{q_x}|^2 \rangle / r_v^3$ , the data is in fact  $\ell_c \langle |\tilde{h}_{q_x}|^2 \rangle / (1000 r_v^2)$  when all lengths are measured in nanometers. We thus scale their  $x$ -axis by  $1/r_v$  and their  $y$ -axis by  $1000 r_v^2$ .

***Analysis of Takatori & Sahu (Phys. Rev. Lett., 2020)***

Figure 1 of Takatori & Sahu [9] reports, in our notation,  $\ell_c \langle |\tilde{h}_{q_x}|^2 \rangle / r_v^3$  versus  $m = q_x r_v$ . In the present study, we take the passive vesicle data and respectively scale the  $x$ -axis and  $y$ -axis by  $1/r_v$  and  $r_v^3$ .

***Analysis of Vutukuri et al. (Nature, 2020)***

An active vesicle is shown in Fig. 1(g) of Vutukuri et al. [10], and is stated to have a surface tension  $\lambda_c = 0.025$  pN/nm. With a bending modulus  $k_b = 42k_B\theta = 174$  pN·nm, we determine  $q_0^- = 8.8 \cdot 10^{-3}$  nm<sup>-1</sup>. Moreover, with a vesicle radius  $r_v \approx 10^4$  nm,  $q_x = m/r_v$  is less than  $q_0^-$  for  $m = \{1, 2, \dots, 88\}$ . Thus, the first 88 modes lie outside the dome and should be excluded from the determination of membrane material properties. We are curious to see where the first 88 modes would fall in Fig. 5 the main text. Unfortunately, the high-tension fluctuation data is—to the best of our knowledge—not publicly available.

**References**

- [1] Sahu, A., Sauer, R. A. & Mandadapu, K. K. [Irreversible thermodynamics of curved lipid membranes](#). *Phys. Rev. E* **96**, 042409 (2017). arXiv:[1701.06495](#).
- [2] Alkadri, A. M. & Mandadapu, K. K. [Irreversible thermodynamics of curved lipid membranes. II. Permeability and osmosis](#). *Phys. Rev. E* **112**, 034413 (2025). arXiv:[2412.19300](#).
- [3] Chandrasekhar, S. *Hydrodynamic and Hydromagnetic Stability* (Dover, New York, 1981).
- [4] Sahu, A., Glisman, A., Tchoufag, J. & Mandadapu, K. K. [Geometry and dynamics of lipid membranes: The Scriven–Love number](#). *Phys. Rev. E* **101**, 052401 (2020). arXiv:[1910.10693](#).
- [5] Pécéréaux, J., Döbereiner, H.-G., Prost, J., Joanny, J.-F. & Bassereau, P. [Refined contour analysis of giant unilamellar vesicles](#). *Eur. Phys. J. E* **13**, 277–290 (2004).
- [6] Faizi, H. A., Reeves, C. J., Georgiev, V. N., Vlahovska, P. M. & Dimova, R. [Fluctuation spectroscopy of giant unilamellar vesicles using confocal and phase contrast microscopy](#). *Soft Matter* **16**, 8996–9001 (2020). arXiv:[2005.09715](#).
- [7] Rautu, S. A. *et al.* [The role of optical projection in the analysis of membrane fluctuations](#). *Soft Matter* **13**, 3480–3483 (2017). arXiv:[1511.05064](#).
- [8] Park, M., Lee, K. & Granick, S. [Response of vesicle shapes to dense inner active matter](#). *Soft Matter* **18**, 6419–6425 (2022).
- [9] Takatori, S. C. & Sahu, A. [Active contact forces drive non-equilibrium fluctuations in membrane vesicles](#). *Phys. Rev. Lett.* **124**, 158102 (2020). arXiv:[1911.01337](#).
- [10] Vutukuri, H. R. *et al.* [Active particles induce large shape deformations in giant lipid vesicles](#). *Nature* **586**, 52–56 (2020).
